# Supplementary material for: Entanglement Entropy and Mutual Information Production Rates in Acoustic Black Holes
Source: arXiv:1101.3272 source file (2011-01-17)
Supplement: Supplementary file 1 [file SupplementalMaterial.pdf]

# Supplemental material for "Entanglement Entropy and Mutual Information Production Rates in Acoustic Black Holes"

Stefano Giovanazzi
*Kirchhoff Institut für Physik, University of Heidelberg, Im Neuenheimer Feld 227, 69120 Heidelberg*

This supplementary material regards some thermodynamic aspects of one-dimensional (1D) ultra-cold degenerate gases flowing through a channel. Some details of non-equilibrium thermodynamics in a generic flowing fluid of spin-less particles are reported. In particular, the classical particle fluctuations formula is generalized to the case of a single channel in contact with two reservoirs at different temperatures including finite size effects. The results are then applied to the case of acoustic black holes.

## I. PARTICLES FLUCTUATIONS IN SINGLE-CHANNEL ACOUSTIC BLACK HOLES

This section contains the derivation of equation (16) of the Letter to which this supplemental material belongs. Such equation relates the fluctuations of the number of particle with Hawking temperature. Here, the classical result for fluctuations at equilibrium is first extended to the non-equilibrium situation of one channel in contact with two reservoirs at different temperatures (subsection I A). Finite size effects are also included. The theory is then applied to the case of a acoustic black hole (also referred to sonic black hole) in Section I B. As a by-product of the calculation, an approximate treatment for the effect of a small initial temperature of the fluid on the particle fluctuations is obtained.

### A. Non-equilibrium particles-fluctuations in a single ballistic channel

The following assumptions are made through this subsection: i) A single one-dimensional channel connecting two reservoirs at different temperatures; ii) The channel supports a finite stationary particle current; iii) In the limit of long wavelengths, the elementary excitation spectrum is saturated by a single sound mode for each direction, i.e. the left-moving and right-moving branches. iv) The sound is characterized by a single speed of sound in a fluid co-moving reference frame. v) The flow is subsonic; vi) The temperatures are sufficiently low that the particle fluctuations on large segments are dominated by thermally excited sound waves, i.e. both the left $kT_L$ and the right $kT_R$ reservoir temperatures are much smaller than $mc^2$, where $c$ is the speed of sound.

The purpose in this subsection is to obtain an expression for the particle fluctuations $\delta N_A^2$ on a macroscopic segment $A$ under the assumptions stated above. The second moment of the particle fluctuations statistics $\delta N_A^2$ is defined by

$$\delta N_A^2 = \Sigma_i p(i) \langle i | \delta \hat{N}_A^2 | i \rangle \qquad (1)$$

where $p(i)$ represents the occupation probability of the state $|i\rangle$ at temperature $kT$ in the canonical ensemble. Such probability is given by $p(i) = \exp(-E_i/kT)/Z$ where $E_i$ is the excitation energy and $Z$ the partition function. The number fluctuation operator in $A$ is defined as $\delta\hat{N}_A = \hat{N}_A - N_A$ where $N_A = \langle \hat{N}_A \rangle$ is the expectation value of the number operator $\hat{N}_A$. $\hat{N}_A$ is related to the density operator $\hat{\rho}(x)$ at position $x$ by $\hat{N}_A = \int_A \hat{\rho}(x) dx$.

The fluctuations $\delta N_A^2$ can be also written as

$$\delta N_A^2 = \int_A dx \int_A dx' \;\; \delta\rho^{(2)}(x', x) \qquad (2)$$

where $\delta\rho^{(2)}(x', x)$ is the two-particle correlation function defined by $\delta\rho^{(2)}(x', x) = \langle \hat{\rho}(x')\hat{\rho}(x) \rangle - \rho(x')\rho(x)$ with the average symbol $\langle \;\; \rangle$ denoting $\Sigma_i p(i) \langle i | \;\; | i \rangle$. Let us consider for simplicity an homogeneous translational invariant system for which $\rho(x)$ is a constant $\rho$ and the two-particle correlation function defined by $\delta\rho^{(2)}(x', x)$ is function only of the difference of the coordinate $x' - x$. It is customary to introduce the correlation function $\nu$ as $\delta\rho^{(2)}(x', x) = \rho\nu(x' - x)$. The static structure factor $S(q)$ and the correlation function $\nu$ are related to each other by the Fourier transform and his inverse

$$S(q) = \int \nu(x) \exp(-iqx)\, dx \qquad (3)$$

$$\nu(x) = \int S(q) \exp(iqx)\, \frac{dq}{2\pi} \qquad (4)$$

Therefore, using the above in the definition (2) we obtain a general relation between the static structure factor $S(q)$ and $\delta N_A^2$

$$\delta N_A^2 = N_A \int S(q) \frac{2\sin^2(Lq/2)}{\pi\, Lq^2}\, dq \qquad (5)$$

where $L$ is the length of the segment $A$. In the integrand of the above equation the factor $2\sin^2(Lq/2)/\pi\, Lq^2$ behaves like a $\delta(q)$ for large $L$. If the static structure factor is finite and well behaving around $q = 0$ then

$$\lim_{L\to\infty} \frac{\delta N_A^2}{N_A} = S(0) \qquad (6)$$

Thus, the $q = 0$ value of the static structure factor measures the particle number squeezing $\delta N_A^2/N_A$ in an ideally infinite large segment. Indeed, at finite temperature

where

$$S(0) = \frac{kT}{mc^2} \tag{7}$$

the use of the asymptotic formula (6) allows us to recover the classical result for the fluctuations

$$\frac{\delta^2 N}{N} = \frac{kT}{mc^2} \tag{8}$$

Thus at finite temperature the length scale to which the system starts behaving macroscopic is given by $l_T = \hbar c/kT$.

For finite value of $L$ finite size effects can be important, especially in the case of zero temperature where $S(0) = 0$ and therefore the asymptotic result is null. In fact, at zero temperature the static structure factor goes to zero linearly in $q$ and his small $q$ behavior is given by

$$S(q) = \frac{1}{2}\xi|q| \tag{9}$$

where $\xi = \hbar/mc$. The integral (5) takes contributions from all hydrodynamic $q$'s and need a cutoff $q_c$

$$\delta N_A^2 = N_A \xi \int_{-q_c}^{q_c} \frac{\sin^2(Lq/2)}{\pi\, L|q|}\, dq \tag{10}$$

$$= N_A \frac{\xi \log(Lq_c)}{\pi L} \tag{11}$$

to logarithmic accuracy. The cutoff value $q_c$ can be taken to be equal to about $2/\xi$, which is a crude estimation of where the static structure factor start to be constant and approach the uncorrelated value of $S(q)$ equal to 1.

For more reading on such finite size corrections to the particle fluctuations in a superfluid see for instance G. E. Astrakharchik, R. Combescot, and L. P. Pitaevskii, Phys. Rev. A **76**, 063616 (2007).

The relationship between $S(q)$ and the fluctuations on a finite segment can be perhaps better seen by inspecting the equivalent definition of the static structure factor given by

$$S(q) = \frac{1}{N}\Sigma_i p(i)\langle i|\delta\hat{\rho}_q \delta\hat{\rho}_q^\dagger|i\rangle \tag{12}$$

where $\hat{\rho}_q^\dagger = \int \exp(iqx)\hat{\rho}(x)$ is the Fourier transform of the density operator. Indeed, the main difference between the definition of the fluctuation in $A$ and the static structure factor in the limit of zero momenta ($q = 0$ limit) is originated from the difference between the operator $\hat{\rho}_0 = \int \hat{\rho}(x)dx$ corresponding to the total number of particles and $N_A = \int_A \hat{\rho}(x)dx$ which corresponds to the number of particles in the region $A$.

Expression (5) and his asymptotic formula (6) are valid also in a non-equilibrium stationary situation. While (5) is quite general, (6) requires probable some regularity of $S(q)$. In the situation of interest of this subsection $S(q)$ is indeed sufficient regular as detailed below.

The static structure factor $S(q)$ receives two independent contributions in the long wavelength limit: One from the left-moving sound waves and the other from the right-moving one. In order to quantify the two contributions it is convenient to start discussing first the dynamic structure factor $S(q,\omega)$ in the single mode approximation (Feynman formula). At zero temperature and positive momentum transfer ($q > 0$) only the right moving sound waves can be excited and $S(q,\omega)$ reads $S(q,\omega) = S_0(q)\delta[\omega - (c+v)q]$ with fluid velocity $v$ and where $S_0(q)$ is the zero-temperature static structure factor in the co-moving reference frame, given by $S_0(q) = \xi q/2$, since the static structure factor (like a snapshot) is a quantity that does not depend on the velocity of the reference frame. For negative momentum transfer ($q < 0$) the dynamic structure factor should instead be given by $S(q,\omega) = S_0(q)\delta[\omega + (c-v)q]$. At finite temperatures of the left or right moving wave branches the previous expressions should be modified to include the stimulated absorption and emission. Therefore, the dynamic structure factor is given by

$$S(q,\omega) = S_0(q)(1+n_{T_L})\delta[\omega + (c+v)q] + S_0(q)\, n_{T_R}\, \delta[\omega - (c-v)q] \qquad \text{for } q > 0 \tag{13}$$

$$S(q,\omega) = S_0(q)(1+n_{T_R})\delta[\omega - (c-v)q] + S_0(q)\, n_{T_L}\, \delta[\omega - (c+v)q] \qquad \text{for } q < 0 \tag{14}$$

where $n_{T_L}$ and $n_{T_R}$ are the boson occupation numbers of the left-moving and right-moving sound modes that are given by

$$n_{T_L} = \frac{1}{\exp\left[\frac{\hbar(c+v)q}{kT_L}\right] - 1} = \frac{1}{\exp(l_L q) - 1} \tag{15}$$

$$n_{T_R} = \frac{1}{\exp\left[\frac{\hbar(c-v)q}{kT_R}\right] - 1} = \frac{1}{\exp(l_R q) - 1} \tag{16}$$

where we have introduced the left and right thermal lengths

$$l_L = \frac{\hbar(c+v)}{kT_L} \tag{17}$$

$$l_R = \frac{\hbar(c-v)}{kT_R} \tag{18}$$

The static structure factor that is the integral of the dynamic structure factor in the frequency domain is given by

$$S(q) = S_0(q)(1 + n_{T_L} + n_{T_R}) \tag{19}$$

In the long wavelength limit and for finite values of the temperatures, the boson occupation numbers $n_{T_L}$ and $n_{T_R}$ are given by

$$n_{T_L} = \frac{kT_L}{\hbar(c+v)q} \gg 1 \tag{20}$$

$$n_{T_R} = \frac{kT_R}{\hbar(c-v)q} \gg 1 \tag{21}$$

$$\tag{22}$$

Therefore, the long wavelength limit of the static structure factor is given by

$$S(q) = \frac{1}{2}\xi q \left[\frac{kT_L}{\hbar(c+v)q} + \frac{kT_R}{\hbar(c-v)q}\right] \tag{23}$$

$$= \frac{kT_L}{2mc(c+v)} + \frac{kT_R}{2mc(c-v)} \tag{24}$$

which translates directly into the final fluctuation formula given by

$$\frac{\delta^2 N}{N} = \frac{kT_L}{2mc(c+v)} + \frac{kT_R}{2mc(c-v)} \tag{25}$$

This espression reduces to the classical equilibrium formula for $v = 0$ and $kT_R = kT_L$.

We consider now finite size effects such those of Eq. (11) which could be observed in an experiment and should be taken into account. These can be estimated by evaluating the integral (5) using the non-equilibrium static factor (19) analogously to the integral (10) and are given by

$$\begin{aligned}\frac{\delta^2 N}{N} &= \frac{\xi}{2\pi L}\ln\left[\frac{l_\mathrm{R}}{\pi L}\sinh\left(\frac{\pi L}{l_\mathrm{R}}\right)\right] \\ &+ \frac{\xi}{2\pi L}\ln\left[\frac{l_\mathrm{L}}{\pi L}\sinh\left(\frac{\pi L}{l_\mathrm{L}}\right)\right] \\ &+ \frac{\xi}{\pi L}\ln\left(Lq_c\right)\end{aligned} \tag{26}$$

### B. Application to acoustic black holes

In order to apply (25) for the evaluation of the particle fluctuations in the subsonic part of a acoustic black hole we need to further assume that: i) The channel is very smooth so that scattering of sound waves is negligible; ii) The channel can be effectively viewed as connecting two reservoirs one of which is at the Hawking temperature $kT_{bh}$ and the other one at the temperature $kT$ of the reservoir from which the particles are originated. Both temperatures are assumed much lower than $mc^2$. iii) Moreover, we shall assume that $kT$ is so low that it does not affect significantly the physics on the sonic horizon and thus Hawking temperature $kT_{bh}$ is still given by Hawking formula (2) of the Letter evaluated with hydrodynamic parameters at zero temperature.

For the evaluation of the particle fluctuations in the supersonic part of a sonic black hole, the only difference is that one need to recognize that the excitation spectrum of the upstream sound mode becomes negative and consequently his temperature appears the negative of the Hawking temperature.

Moving the attention towards the practical application, the number-of-particle fluctuations in subsonic segment $A$ and in the supersonic segment $B$ are asymptotically given by

$$\frac{\delta^2 N_A}{N_A} = \frac{kT}{2mc_A(c_A+v_A)} + \frac{kT_{bh}}{2mc_A(c_A-v_A)} \tag{27}$$

$$\frac{\delta^2 N_B}{N_B} = \frac{kT}{2mc_B(c_B+v_B)} + \frac{kT_{bh}}{2mc_B(v_B-c_B)} \tag{28}$$

where $N_A$ and $N_A$ are the average particle number in $A$ and $B$, respectively. Since in general both $v$ and $c$ differ between subsonic and supersonic regions, the measurement of such fluctuations provides in principle a way to extract both $kT_{bh}$ and the fluid reservoir temperature $kT$ as well as the corresponding entropies. Moreover, by applying an external potential difference between $A$ and $B$, the velocities entering in (27) and (28) can be further tuned without changing $kT$ and $kT_{bh}$, thus offering an extra knob to the experimentalist.

Equations (27) and (28) should be compared with Equation (28) of the Letter, which is reproduced below for completeness

$$\frac{\delta N_A \delta N_B}{\sqrt{N_A N_B}} = -\frac{kT_{bh}}{2m\sqrt{c_A(c_A-v_A)c_B(v_B-c_B)}} \tag{29}$$

The correlation between particle number fluctuations $\delta N_A$ and $\delta N_B$ should be in first approximation independent on the reservoir initial temperature.
